# Supplementary material for: Generating Object Stamps
Source: arXiv:2001.02595 source file (2020-01-10)
Supplement: Supplementary file 1 [file supplemental_old.tex]

\RequirePackage{snapshot} %Lists all dependencies
\documentclass[10pt,twocolumn,letterpaper,table]{article}

\usepackage{../cvpr}
\usepackage{times}
\usepackage{epsfig}
\usepackage{graphicx}
\usepackage{amsmath}
\usepackage{amssymb}
\usepackage{tikz}
\usepackage{enumitem}
% \usepackage{xcolor}
% \usepackage [table]{xcolor}
\usepackage{authblk}
\include{includes}

% Include other packages here, before hyperref.

% If you comment hyperref and then uncomment it, you should delete
% egpaper.aux before re-running latex.  (Or just hit 'q' on the first latex
% run, let it finish, and you should be clear).
\usepackage[pagebackref=true,breaklinks=true,colorlinks,bookmarks=false]{hyperref}

%\cvprfinalcopy % *** Uncomment this line for the final submission

\def\cvprPaperID{4236} % *** Enter the CVPR Paper ID here
\def\httilde{\mbox{\tt\raisebox{-.5ex}{\symbol{126}}}}




% Pages are numbered in submission mode, and unnumbered in camera-ready
%\ifcvprfinal\pagestyle{empty}\fi
%\setcounter{page}{4321}
\begin{document}

%%%%%%%%% TITLE
\title{Exploring the Spectrum of Mask Supervision\\for Unpaired Image-to-Image Translation \\ Supplementary Material
%From Supervised to Unsupervised Unpaired Image-to-Image Image Translation \\ 
%Good Enough GAN: The Unreasonable Effectiveness of Weak Segmentation in Unpaired Image-to-Image Translation. \\
%(I Can't Get No) Supervision \dots in Unpaired Image-to-Image Translation
}
%\title{Unreasonable Mask Supervision for Unpaired Image-to-Image Object Transformation}
%\title{The Spectrum of Supervision for Unpaired Object-to-Object Image Transformation}

% \author{First Author\\
% Institution1\\
% Institution1 address\\
% {\tt\small firstauthor@i1.org}
% % For a paper whose authors are all at the same institution,
% % omit the following lines up until the closing ``}''.
% % Additional authors and addresses can be added with ``\and'',
% % just like the second author.
% % To save space, use either the email address or home page, not both
% \and
% Second Author\\
% Institution2\\
% First line of institution2 address\\
% {\tt\small secondauthor@i2.org}
% }


\author[1]{Aaron Gokaslan\thanks{Equal Contribution}}
\author[2]{Youssef A. Mejjati\protect\footnotemark[1]}
\author[3]{Oliver Wang}
\author[2]{Kwang In Kim}
\author[1]{James Tompkin}
\makeatletter
\renewcommand\AB@affilsepx{, \protect\Affilfont}
\makeatother
\affil[1]{Brown University}\affil[2]{University of Bath}\affil[3]{Adobe}

% \input{src/figures/teaser}


\maketitle

% \begin{abstract}
% Current unsupervised image-to-image translation techniques have proven to struggle when faced with domains exhibiting significant shape changes. 
% Recently proposed approaches enable this property but require instance-level segmentations which limit their domain applicability due to the cost of acquiring this supervision.
% We explore and analyze the effect of different forms of supervised masks for image-to-image translation under significant shape change. 
% We show qualitatively and quantitatively that imprecise supervisions can produce appealing results, sometimes comparable to the full-supervision case.
% \end{abstract}

\section{Network Architectures}
\label{sec:Architecture}

Our networks are constructed from similar components to Cycle
GAN~\cite{zhu2017unpaired}. The encoder consists of three convolutional downsampling layers and nine residual blocks (Table~\ref{tab:Gencodingarchitecture}). The decoding architecture of the generator is given by Table~\ref{tab:Gdecoderarchitecture}. 

The discriminator also consists of a similar encoder-decoder structure. The encoding architecture is in this case give in Table~\ref{tab:Dencoderarchitecture}, while the decoder is given in Table~\ref{tab:Ddecodingarchitecture}.
% \import{\tabDir}{architecture_table}
\import{\tableDir}{architecture_table}

\section{Systems}
All experiments were run using either two NVidia 1080 GPUs or a single NVidia 1080 Ti GPU, written in Tensorflow~\cite{tensorflow2015-whitepaper} using the Tensorpack~\cite{wu2016tensorpack} library. We will release our code and data as open source.

\section{Additional results}
\label{sec:Additional results}
We show qualitative results on the Airplane and Bird dataset for their bidirectional translations (Figure~\ref{tab:absupervision}) as well as Horse to Zebra dataset (Figure~\ref{tab:hzsupervision}); plus additional qualitative results for the datasets used in the main paper (Giraffe and Sheep---Figure~\ref{tab:gssupervision}; Bear and Elephant---Figure~\ref{tab:besupervision}; Toilet and Fire Hydrant---Figure~\ref{tab:ftsupervision}). All images shown are drawn from the test dataset; we sample images at different object scales and with different object configurations to provide a representation of overall result quality. We also reject images with close-ups, e.g., where we see only the wing of a plane or only the face of a sheep.

For the special case of Fire Hydrant to Toilet (Figure~\ref{tab:ftsupervision}), we notice that the background endures severe changes, moreover the generated foreground does not generally blend correctly with the background. This is because these specific classes (Fire Hydrant and Toilet) are generally present in completely different scenes: the first one is on the street while the second one is in a restroom. Such environment discrepancy obliges the generator to heavily alter the background in order to convince the corresponding discriminator.
\import{\figDir}{supervisionlevels_supplemental}
 
% \ow{add horse to zebra results as well, to show that our method is actually comparable on that task}\ym{On it as soon as we have the data.}
 
% \kimki{I wonder what kind of discussion we could add about  Fig.~\ref{tab:ftsupervision}.Unlike other examples, here the background scene context where the transferred objects appear seem to be significantly different from the original scene context. I understand that no transfer algorithm considered here explicitly model how the transferred foregrounds are `naturally blend' in the scene context; but they would do that indirectly depending on how the discriminators are configured? Are these algorithms struggling to inpaint backgrounds in a way that the transferred objects match them?} \jt{we have a bit of this discussion in the main paper - should we add to it here?}
 
{\small
\bibliographystyle{ieee}
\bibliography{segmentgan}
}

\end{document}
